# Supplementary material for: Cycle-Consistent Counterfactuals by Latent Transformations
Source: arXiv:2203.15064 source file (2022-03-28)
Supplement: Supplementary file 1 [file misc.tex]

% ------------------------------------------------------------------
\begin{table*}[ht]
\caption{Normalized Counterfactual Transition Scores.}
\label{table:cout_norm_supp}
% \vskip 0.05in
\begin{center}
\begin{small}
\resizebox{\textwidth}{!}{%

\begin{tabular}{l|cc|cc|cc|cc|cc}

{\sc Methods} & 
\multicolumn{2}{c|}{ExpGAN COMP\cite{samangouei2018explaingan}} &
\multicolumn{2}{c|}{ExpGAN CF\cite{samangouei2018explaingan}} &
\multicolumn{2}{c|}{CEM\cite{dhurandhar2018explanations}}  &
\multicolumn{2}{c|}{CVE \cite{goyal2019counterfactual}} & 
\multicolumn{2}{c}{CFL (ours)}\\
\cline{1-11}
{}  &   Mnist&FMnist  &  Mnist&FMnist  &  Mnist&FMnist  &  Mnist&FMnist  &  Mnist&FMnist\\ 
\cline{2-11}
{$AUPC_{c'}\uparrow$}   &  {$0.972\pm0.02$}&{$0.935\pm0.02$}  &  {$0.962\pm0.02$}&{$0.940\pm0.05$}  &  {$\bb{0.990\pm0.01}$}&{$\bb{0.965\pm0.01}$}  &   {$0.253\pm0.02$}&{$0.365\pm0.04$}  &  {$0.982\pm0.01$}&{$0.939\pm0.01$}\\ 

{$AUPC_{c}\downarrow$}  &  {$0.038\pm0.01$}&{$0.060\pm0.01$}  &  {$0.045\pm0.01$}&{$0.081\pm0.02$}  &  {$0.047\pm0.016$}&{$\bb{0.055\pm0.00}$}  &  {$0.728\pm0.01$}&{$0.602\pm0.04$}  &  {$\bb{0.031\pm0.01}$}&{$0.059\pm0.00$}\\ 

\cline{2-11}
{$COUT\uparrow$}        &  {$0.934\pm0.03$}&{$0.875\pm0.03$}  &  {$0.917\pm0.03$}&{$0.859\pm0.06$}  &  {$0.943\pm0.010$}&{$\bb{0.910\pm0.01}$}  &  {$-0.475\pm0.033$}&{$-0.237\pm0.08$}  &  {$\bb{0.951\pm0.03}$}&{$0.879\pm0.02$}
\end{tabular}
}
\end{small}
\end{center}
% \vskip -0.25in
\end{table*}
% ------------------------------------------------------------------

% ------------------------------------------------------------------
\begin{table*}[ht]
\caption{Counterfactual Transition Scores.}
\label{table:cout_supp}
% \vskip 0.05in
\begin{center}
\begin{small}
\resizebox{\textwidth}{!}{%

\begin{tabular}{l|cc|cc|cc|cc|cc}

{\sc Methods} & 
\multicolumn{2}{c|}{ExpGAN COMP\cite{samangouei2018explaingan}} &
\multicolumn{2}{c|}{ExpGAN CF\cite{samangouei2018explaingan}} &
\multicolumn{2}{c|}{CEM\cite{dhurandhar2018explanations}}  &
\multicolumn{2}{c|}{CVE \cite{goyal2019counterfactual}} & 
\multicolumn{2}{c}{CFL (ours)}\\
\cline{1-11}  
{}  &   Mnist&FMnist &  Mnist&FMnist   &   Mnist&FMnist &  Mnist&FMnist  &  Mnist&FMnist\\ 
\cline{2-11}
{$AUPC_{c'}\uparrow$}  &  {$0.967\pm0.02$}&{$0.920\pm0.01$}  &  {$0.960\pm0.01$}&{$0.675\pm0.15$}  &  {$0.30\pm0.10$}&{$0.347\pm0.07$}  &  {$0.21\pm0.02$}&{$0.275\pm0.03$}  &  {$\bb{0.980\pm0.02}$}&{$\bb{0.936\pm0.02}$}\\ 

{$AUPC_{c}\downarrow$} &  {$0.040\pm0.01$}&{$0.062\pm0.01$}  &  {$0.045\pm0.01$}&{$0.091\pm0.03$}      &   {$0.55\pm0.18$}&{$0.427\pm0.01$}   &    {$0.77\pm0.01$}&{$0.638\pm0.04$}  &  {$\bb{0.031\pm0.02}$}&{$\bb{0.058\pm0.01}$}\\ 

\cline{2-11}
{$COUT\uparrow$}       &  {$0.927\pm0.03$}&{$0.858\pm0.02$}  &  {$0.915\pm0.03$}&{$0.583\pm0.16$}      &   {$-0.25\pm0.26$}&{$-0.080\pm0.06$}   &    {$-0.56\pm0.34$}&{$-0.363\pm0.07$} &  {$\bb{0.948\pm0.03}$}&{$\bb{0.877\pm0.02}$}
\end{tabular}
}
\end{small}
\end{center}
% \vskip -0.25in
\end{table*}
% ------------------------------------------------------------------

% ------------------------------------------------------------------
\begin{table*}[ht]
\caption{Feasibility of the Generated Counterfactuals.}
\label{table:val_supp}
% \vskip 0.05in
\begin{center}
\begin{small}
\resizebox{\textwidth}{!}{%
\begin{tabular}{l|cc|cc|cc|cc|cc}

{\sc Methods} & 
\multicolumn{2}{c|}{ExpGAN COMP\cite{samangouei2018explaingan}} & 
\multicolumn{2}{c|}{ExpGAN CF\cite{samangouei2018explaingan}} & 
\multicolumn{2}{c|}{CEM \cite{dhurandhar2018explanations}} & 
\multicolumn{2}{c|}{CVE\cite{goyal2019counterfactual}} & 
\multicolumn{2}{c}{CFL (ours)}\\
\cline{1-11}
{}                  &   Mnist&FMnist  &  Mnist&FMnist  &  Mnist& FMnist  &  Mnist& FMnist  &  Mnist& FMnist \\
\cline{2-11}
{$val\uparrow$}     &  {$0.997\pm0.002$}&{$0.998\pm0.001$}  &  {$0.998\pm0.002$}&{$0.776\pm0.160$}  &  {$0.468\pm0.246$}&{$0.620\pm0.128$}       &  $0.231\pm0.125$&{$0.145\pm0.078$}  &  {$\bb{0.999\pm0.000}$}&{$1.0\pm0.0$}\\ 

{$prox\downarrow$}  &  {$0.074\pm0.023$}&{$0.135\pm0.040$}  &  {$0.133\pm0.026$}&{$0.255\pm0.012$}  &  {$\bb{0.016\pm0.002}$}&{$0.013\pm0.002$}  &  $0.055\pm0.002$&{$0.054\pm0.003$}  &  {$0.072\pm0.016$}&{$0.116\pm0.027$}\\ 

{$sprs\downarrow$}  &  {$0.163\pm0.036$}&{$0.406\pm0.022$}  &  {$0.285\pm0.034$}&{$0.680\pm0.072$}  &  {$\bb{0.066\pm0.009}$}&{$0.132\pm0.018$}  &  $0.167\pm0.009$&{$0.263\pm0.008$}  &  {$0.246\pm0.017$}&{$0.973\pm0.007$}
\end{tabular}
}
\end{small}
\end{center}
% \vskip -0.25in
\end{table*}
% ------------------------------------------------------------------

% ------------------------------------------------------------------
\begin{table*}[ht]
\caption{Realism of the Generated Counterfactuals.}
\label{table:real_supp}
% \vskip 0.05in
\begin{center}
\begin{small}
\resizebox{\textwidth}{!}{%
\begin{tabular}{l||cc|cc|cc|cc|cc||cc|cc}

{\sc Methods} & 
\multicolumn{2}{c||}{ExpGAN COMP\cite{samangouei2018explaingan}} & 
\multicolumn{2}{c||}{ExpGAN CF\cite{samangouei2018explaingan}} & 
\multicolumn{2}{c|}{CEM\cite{dhurandhar2018explanations}} &
\multicolumn{2}{c|}{CVE\cite{goyal2019counterfactual}}& 
\multicolumn{2}{c||}{CFL (ours)}&
\multicolumn{2}{c|}{Original data}& 
% \multicolumn{2}{c|}{Generated data}& 
\multicolumn{2}{c}{Adversarial data}\\

\cline{1-15}
{}                 &  Mnist&FMnist  &  Mnist&FMnist  &  Mnist&FMnist  &  Mnist&FMnist  &  Mnist&FMnist  &  Mnist&FMnist  &  Mnist&FMnist  \\%&  Mnist&FMnist \\ 
\cline{2-15}
{$IM1\downarrow$}           &   {$0.72\pm0.07$}&{$0.77\pm0.12$}  &  {$0.45\pm0.11$}&{$0.67\pm0.11$}  &  {$1.68\pm0.32$}&{$1.62\pm0.31$}  &  {$1.44\pm0.17$}&{$1.24\pm0.05$}  &  {${0.70\pm0.08}$}&{$0.76\pm0.30$}  &  {$0.46\pm0.09$}&{$0.57\pm0.13$}  &  {1.303}&{-- --}\\ 

{$IM2\times 10\downarrow$}  &   {$0.43\pm0.07$}&{$0.14\pm0.01$}  &  {$0.30\pm0.27$}&{$0.14\pm0.03$}  &  {$1.08\pm0.34$}&{$0.26\pm0.13$}   &   {$1.38\pm0.27$}&{$0.37\pm0.14$}  &  {${0.36\pm0.09}$}&{$0.096\pm0.04$}  &  {$0.29\pm0.04$}&{$0.11\pm0.01$}  &  {0.831}&{-- --}\\ 

{$FID\downarrow$}           &   {$56.26\pm1.62$}&{$88.97\pm1.53$}  &  {$34.83\pm0.42$}&{$129.15\pm2.32$}  &  {$60.73\pm1.25$}&{$105.84\pm2.15$}  &  {$69.46\pm1.44$}&{$93.57\pm1.10$}  &  {$\bb{30.7\pm1.04}$}&{$--$}  &  {$14.47\pm0.20$}&{$27.47\pm0.55$}  &  {-- --}&{-- --}
\end{tabular}
}
\end{small}
\end{center}
% \vskip -0.25in
\end{table*}
% ------------------------------------------------------------------
